# Supplementary material for: SegNeXt: Rethinking Convolutional Attention Design for Semantic Segmentation
Source: arXiv:2209.08575 source file (2022-09-18)
Supplement: Supplementary file 1 [file Supplementary.tex]

% \documentclass{article}

% % if you need to pass options to natbib, use, e.g.:
% \PassOptionsToPackage{numbers, compress}{natbib}
% % before loading neurips_2021

% % ready for submission

% \usepackage{neurips_2022}

% % to compile a preprint version, e.g., for submission to arXiv, add add the
% % [preprint] option:
% % \usepackage[preprint]{neurips_2022}

% % to compile a camera-ready version, add the [final] option, e.g.:
% %     \usepackage[final]{neurips_2021}

% % to avoid loading the natbib package, add option nonatbib:
% %    \usepackage[nonatbib]{neurips_2021}

% % \usepackage{hyperref}       % hyperlinks
% \usepackage{url}            % simple URL typesetting
% \usepackage{amsfonts}       % blackboard math symbols
% \usepackage{nicefrac}       % compact symbols for 1/2, etc.
% \usepackage{microtype}      % microtypography
% \usepackage[dvipsnames,table,xcdraw]{xcolor}
% \usepackage{graphicx}
% \usepackage{amsmath,amssymb} % define this before the line numbering.
% \usepackage{booktabs}

% \usepackage{overpic}


% \usepackage{multirow}
% \newcommand{\tabincell}[2]{\begin{tabular}{@{}#1@{}}#2\end{tabular}}
% \usepackage{makecell}
% \usepackage{wrapfig}


% \usepackage{pifont}
% \newcommand{\cmark}{\ding{51}}%
% \newcommand{\xmark}{\text{\ding{55}}}


% \usepackage{silence}
% \hbadness=10000 \vbadness=10000 

% \graphicspath{{./Images/}}

% \newcommand{\gmh}[1]{\textcolor{blue}{#1}}
% \newcommand{\lcz}[1]{\textcolor{green}{#1}}
% \newcommand{\gzy}[1]{\textcolor{orange}{#1}}
% \newcommand{\todo}[1]{\textcolor{red}{#1}}
% \newcommand{\hou}[1]{\textcolor{RoyalBlue}{[QB:#1]}}

% \usepackage[pagebackref=false,breaklinks,colorlinks,linkcolor=blue,citecolor=RoyalBlue]{hyperref}

% \def\etal{{\em et al.}}
% \def\aka{\emph{a.k.a.,~}}
% \def\wrt{\emph{w.r.t.,~}}
% \def\sArt{state-of-the-art~}
% \def\ie{\emph{i.e.,~}}
% \def\eg{\emph{e.g.,~}}
% \def\etc{{\em etc}}
% \def\modelname{SegNeXt}

% \newcommand{\addImgs}[1]{}


% \newcommand{\figref}[1]{Fig.~\ref{#1}}
% \newcommand{\tabref}[1]{Tab.~\ref{#1}}
% \newcommand{\secref}[1]{Sec.~\ref{#1}}

% \title{
% Appendix for "SegNeXt: Rethinking Convolutional Attention Design 
% for Semantic Segmentation"
% }

% \begin{document}

% \maketitle

% \section{Training Details}
% We show some training details on different datasets
% omitted in the main paper in~\tabref{Tab.training_details}.
% For different benchmarks, 
% we employ different training settings for fair comparison.

% \begin{table}[htp!]
%   \centering
%   \setlength{\tabcolsep}{2.6mm}
%   \caption{Training details on different benckmarks. 
%   80K + 80K means we pretrain 80K iterations on Pascal VOC trainaug set and finetune 80K on its trainval set.
%   80K + 40K denotes we pretrain 600K iterations on COCO dataset and finetune 40K on its trainval set.}
%   \begin{tabular}{l|c|c|c}
%     \toprule
%     \textbf{Dataset} & \textbf{Crop Size} & \textbf{Batch Size} & \textbf{Iterations}   \\ \midrule
%     ADE20K~\cite{zhou2017scene}          & 512 $\times$ 512  & 16 & 160K \\
%     Cityscapes~\cite{cordts2016cityscapes} & 1,024$\times$1,024 & 8 & 160K  \\
%     COCO-Stuff~\cite{caesar2018coco}       & 512 $\times$ 512 & 16 & 80K  \\ 
%     Pascal VOC~\cite{everingham2010pascal}      & 512 $\times$ 512 & 16 & 80K + 80K  \\ 
%     Pascal VOC~\cite{everingham2010pascal} w/ COCO~\cite{lin2014microsoft}   & 512 $\times$ 512 & 16 & 600K + 40K  \\ 
%     Pascal Context ~\cite{mottaghi2014role}  & 480 $\times$ 480 & 16 & 
%   80K \\ 
%     iSAID~\cite{waqas2019isaid}       & 896 $\times$ 896 & 16 & 160K  \\ 
%     \bottomrule
%   \end{tabular}
%   \label{Tab.training_details}
% \end{table}


% \section{Ablation about MSCA Head}



% In addition to using a variant of self-attention as our head, we also used MSCA as our head. 
% Results in~\tabref{tab:ablation_head} show Ham head~\cite{geng2021attention} achieves a better performance 
% than MSCA head, which demonstrates a CNN-style encoder 
% requires a segmentation head with a global receptive field.

% \begin{table}[htp!]
%     \centering
%     \renewcommand{\arraystretch}{1}
%     \renewcommand{\tabcolsep}{3mm}
%     \caption{Performance of different head in decoder. 
%     SegNeXt-T w/ Ham means the MSCAN-T encoder plus the Ham decoder.
%     FLOPs are calculated using the input size of 512$\times$512.
%     Experiments are conducted on COCO-Stuff dataset.
%     }
%     \begin{tabular}{l|cc|cc}
%         \toprule
%     	Architecture  & Params. (M) & GFLOPs & mIoU (SS) & mIoU (MS)  \\ \midrule
%     	SegNeXt-T w/ MSCA & 4.4 & 6.7 & 38.2 & 38.6 \\ 
%     	SegNeXt-T w/ Ham~\cite{geng2021attention} & 4.3 & 6.6  & 38.7 & 39.1 \\ 
%     	\midrule
%     	SegNeXt-S w/ MSCA & 14.0 & 15.9 & 42.1 & 42.4 \\ 
%     	SegNeXt-S w/ Ham~\cite{geng2021attention} & 13.9 & 15.9 & 42.2 & 42.8 \\ 
%     	\midrule
%     	SegNeXt-B w/ MSCA & 28.0 & 33.6 & 45.1 & 45.5 \\ 
%     	SegNeXt-B w/ Ham~\cite{geng2021attention} & 27.6 & 34.9 & 45.8 & 46.3 \\ 
%     	\midrule
%     	SegNeXt-L w/ MSCA & 50.1 & 69.8 & 45.9 & 46.4 \\ 
%     	SegNeXt-L w/ Ham~\cite{geng2021attention} & 48.9 & 70.0 & 46.5 &
%     	47.2 \\ 
%         \bottomrule
%     \end{tabular}
%     \label{tab:ablation_head}
%     % \vspace{-0.2cm}
% \end{table}




% \section{More Qualitative Results}
% In the main paper, we show the qualitative results
% on Cityscapes dataset. Here, we display qualitative results 
% on ADE20K dataset in ~\figref{fig:vis_ade}.
% The figure clearly shows 
% that our method is better
% at understanding the details.

% \begin{figure}[htp!]
%   \centering %\flushright
%   \footnotesize
%   \begin{overpic}[width=0.95\linewidth]{./Images/vis_ade.pdf}
%   \end{overpic}
% \caption{ Qualitative results on ADE20K dataset. Left: SegFromer-B2. Middle: SegNeXt-B. Right: Ground trurh. }
% \label{fig:vis_ade}
% \vspace{-0.1cm}
% \end{figure}

% \section{Visualization results}

% We adopt Grad-CAM~\cite{selvaraju2017grad} to conduct visualization. 
% As shown in ~\figref{fig:grad_cam}, we can clearly find our MSCAN 
% shows better visualization results. 
% In particular, when object occupies most of area in an image
% (shown in first three columns)
% or multiple objects in an image (shown in last three columns), 
% ConvNeXt~\cite{liu2022convnet} appears inaccurate, 
% while our MSCAN still works well.
% It shows the effectiveness of
% larger receptive field and multi-scale information aggregation.


% \begin{figure}[htp!]
%   \centering %\flushright
%   \footnotesize
%   \begin{overpic}[width=0.95\linewidth]{./Images/cam_segnext.pdf}
%   \end{overpic}
% \caption{ Visualization results by using Grad-CAM~\cite{selvaraju2017grad}. Top: grad-cam figures of ConvNeXt~\cite{liu2022convnet}. Bottom: grad-cam figures of our MSCAN.}
% \label{fig:grad_cam}
% \vspace{-0.1cm}
% \end{figure}




% \bibliographystyle{eccv22.bst}
% \bibliography{neurips_2022}



% \end{document}
